# Supplementary material for: Vectorial observation of the spin Seebeck effect in epitaxial NiFe$_2$O$_4$ thin films with various magnetic anisotropy contributions
Source: arXiv:1902.05384 ancillary file (2019-05-12)
Supplement: Supplementary file 1 [file Zhong_Li_Jan_Krieft_supplementary_material_vector_SSE.pdf]

# Supplementary Material

## Vectorial observation of the spin Seebeck effect in epitaxial $\text{NiFe}_2\text{O}_4$ thin films with various magnetic anisotropy contributions

Zhong Li,<sup>1,2,\*</sup> Jan Kriefft,<sup>3,\*</sup> Amit Vikram Singh,<sup>1</sup> Sudhir Regmi,<sup>1,2</sup> Ankur Rastogi,<sup>1,†</sup> Abhishek Srivastava,<sup>1,2</sup> Zbigniew Galazka,<sup>4</sup> Tim Mewes,<sup>1,2</sup> Arunava Gupta,<sup>1,‡</sup> and Timo Kuschel<sup>3,§</sup>

<sup>1</sup>*Center for Materials for Information Technology,  
The University of Alabama, Tuscaloosa, Alabama 35487, USA*

<sup>2</sup>*Department of Physics & Astronomy,  
The University of Alabama, Tuscaloosa, Alabama 35487, USA*

<sup>3</sup>*Center for Spinelectronic Materials and Devices,  
Department of Physics, Bielefeld University,  
Universitätsstraße 25, 33615 Bielefeld, Germany*

<sup>4</sup>*Leibniz-Institut für Kristallzüchtung, Max-Born-Str. 2, 12489 Berlin, Germany*

(Dated: April 25, 2019)

## I. Sample preparation and SSE setup

$\text{NiFe}_2\text{O}_4$  (NFO) films were deposited on (011)- or (001)-oriented MGO and CGO substrates ( $5 \times 5 \times 0.5 \text{ mm}^3$ ) by pulsed laser deposition (PLD) in an oxygen environment with a background pressure of 10 mTorr. The laser fluence was set to be  $\sim 1 \text{ J/cm}^2$ . The temperature of the substrates was kept constant at  $700^\circ\text{C}$  during film growth. For LSSE measurements, a 5 nm thick Pd film was deposited *in situ* by DC sputtering at 20 W power and 5 mTorr Ar pressure on top of the PLD grown NFO films.

In the setup for LSSE measurements (see Main Text Fig. 1(a)), the samples were sandwiched between two copper blocks. A thermally conducting and electrically insulating  $250 \mu\text{m}$  thick spacer (SiC) was used between the Pd layer and the upper copper block. This SiC spacer is prepared to fit the  $5 \text{ mm}^3$  surface of the Pd leaving a 0.5 mm edge to allow for a clean bonding contact to the Pd-surface on all sides. Therefore, a centering of the upper copper block connected to the spacer is necessary using positioning screws for higher precision. One Peltier module was used to heat up the upper copper block and the other Peltier module was used to cool down the lower copper block to keep it at room temperature (293 K). The temperature of the lower copper block was fixed at a base temperature  $T$ , while the temperature of the upper block ( $T + \Delta T$ ) was varied to obtain the desired temperature gradient across the sample (base temperature  $T$  is set to room temperature 293 K, and  $\Delta T = 20 \text{ K}$  if not stated otherwise). The temperature gradient was measured between the upper and lower copper blocks by two K-type thermocouples. For the angular dependence measurements of LSSE, the whole stack was rotated in-plane with a manual stage. To carry out vectorial LSSE measurements (see Main Text Fig. 1(b)), four aluminum wires were bonded orthogonally on the middle of all four sides of the Pd layer and connected to two separate nanovoltmeters.

## II. X-ray diffraction results

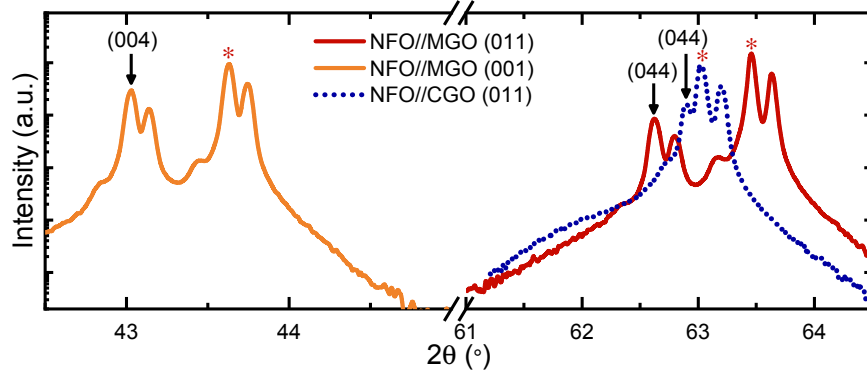

FIG. S1. (Color online) XRD  $\theta - 2\theta$  diffraction patterns of NFO films ( $\downarrow$ ) on different substrates (MGO (011), MGO (001), CGO (011))(\*), respectively. The splitting of the peaks for the films and substrates stem from  $\text{Cu-K}\alpha_1$  and  $\text{Cu-K}\alpha_2$  radiation wavelengths.

Figure S1 shows XRD  $\theta - 2\theta$  scans in the range of  $2\theta = 42^\circ - 46^\circ$  for NFO//MGO (001) displaying (004) diffraction peaks corresponding to substrate and NFO film. The MGO and CGO (011)-oriented films display (044) diffraction peaks in the range of  $2\theta = 61^\circ - 65^\circ$ , respectively. We can observe a larger gap between the film and substrate peak positions for both NFO//MGO samples, while the film peak is nearly merged with the left shoulder of the substrate peak for the NFO//CGO sample, which indicates that the NFO//CGO sample has lower lattice mismatch than NFO//MGO samples.

### III. VSM and SSE results for NFO//MGO (001)

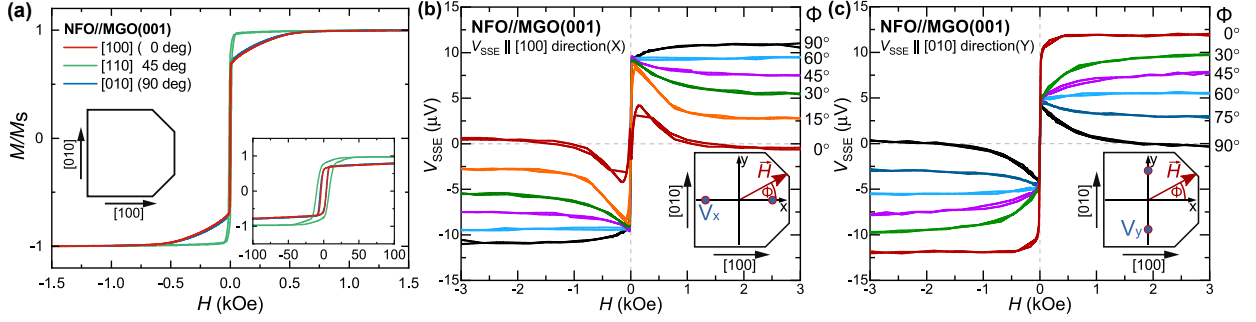

FIG. S2. (Color online) (a) VSM results of the normalized in-plane magnetization versus the magnetic field for NFO//MGO (001). The magnetizations are measured with the in-plane magnetic field applied in two perpendicular ([100] and [010]) and one diagonal [110] directions. (b) (c) LSSE measurements at various angles along two perpendicular directions ([100] and [010]) for NFO//MGO (001), respectively. The represented angles  $\phi$  are the angles between the  $x$  axis and the applied field  $H$  (see schematic in Main Text Fig. 1).

From Fig. S2(a), we see that the shapes of magnetization loops for NFO//MGO (001) thin film along both [010] and [100] directions are comparable, which implies that the thin film has a four-fold magnetic anisotropy without any additional uniaxial magnetic anisotropy. Consequently, as shown in Figs. S2(b) and S2(c), we also find that the shapes of SSE along these two perpendicular directions are similar.

#### IV. Analysis of the voltage $V_{\text{SSE}}$ anisotropy

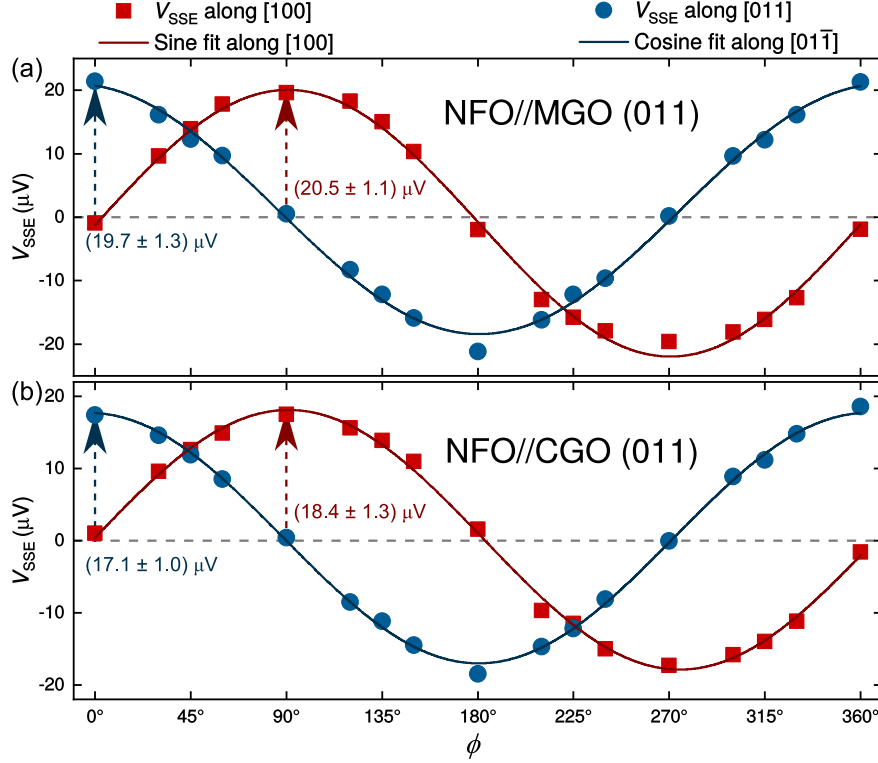

FIG. S3. (Color online) Angle dependence of the voltage  $V_{\text{SSE}}$  measured along the  $[100]$  ( $V_{x,\text{sat}}$ , red) and  $[01\bar{1}]$  ( $V_{y,\text{sat}}$ , blue) direction of (a) NFO/MGO (011) and (b) NFO/CGO (011) at the maximum applied external magnetic field of 3 kOe approaching the saturation value. The amplitude of the SSE voltage is specified for the corresponding fit with an error mainly influenced by the orientation of the external magnetic field ( $\pm 2.5^\circ$ ) and the uncertainty of the fit.

In the Main Text we derive that the material and setup parameter  $A_x$  and  $A_y$  are equal in good approximation for both presented samples and use this to calculate the magnitude and azimuthal angle of the magnetization. Here, we can also choose a broader approach and evaluate the angular dependence of the LSSE saturation voltages  $V_x$  and  $V_y$ . For a sufficiently large external magnetic field we can determine the voltages  $V_x$  and  $V_y$  in saturation ( $V_{x,\text{sat}}$  and  $V_{y,\text{sat}}$ ) and plot those values in relation to the external magnetic field angle  $\phi$ . This fit evaluation is presented in Fig. S3 measured along the  $[100]$  and  $[01\bar{1}]$  direction of the NFO/MGO (011) and NFO/CGO (011) sample.

We can assume that

$$\begin{aligned} V_{x,\text{sat}} &= A_x M_{y,\text{sat}} = A_x M_s \sin \phi & \text{and} \\ V_{y,\text{sat}} &= A_y M_{x,\text{sat}} = A_y M_s \cos \phi \end{aligned} \quad (\text{S1})$$

is valid here and directly see that both voltage amplitudes are comparable in magnitude which confirms our assumption of a strain-independent ISHE. By fitting the data presented in Fig. S3 according to Eq. (S1) one can determine the proper proportionality factors to convert the SSE voltages  $V_x$  and  $V_y$  to  $M_x$  and  $M_y$  according to Eq. (3) of the Main Text including quantitatively obtained values for the parameters  $A_x$  and  $A_y$ . For the presented samples we do not see any deviation of the fitted parameters within the measurement accuracy and therefore  $A_x \approx A_y$  is a valid assumption here. This determination of the proportionality factors is feasible for more complex systems with significantly anisotropic magnon dispersion. Furthermore, by utilizing this approach we would be able to see deviations from saturation in the residual of the fits and can therefore determine a sufficient saturation field. For example, we only see a small deviation from the fits presented in Fig. S3 indicating a nearly saturated state at maximum field.

## V. Vector LSSE measurement results for NFO//CGO (011) and NFO//MGO (001)

As shown in Fig. S4, we present the reversal process of NFO//CGO (011) using the same selected angles of the external magnetic field  $\phi$  in our vectorial magnetometry measurements (see Main Text insert Fig. 2(d)). The NFO//CGO (011) sample shows a dominant fourfold anisotropy with magnetic easy axes along the  $45^\circ$  directions relative to the magnetic harder directions along  $[100]$  and  $[01\bar{1}]$ . Here, we clearly see a switching of the magnetization along or close to the magnetic easy axis. For angles of the external magnetic field in between those magnetic easy directions (Fig. S4(a) and S4(d)), we observe a coherent rotation of the magnetization vector out of the magnetic hard axis followed by a sharp switching by  $180^\circ$ . Subsequently, the magnetization rotates back out of the magnetic easy axis while the external magnetic field is reaching its maximum. Since the uniaxial magnetic anisotropy is relatively weak compared to the one of the NFO//MGO (011) sample, as indicated by the absolute value of the resonance field  $H_{\text{res}}$ , the switching can occur when the magnetization has been rotated up to  $\sim 15^\circ$  relative to the magnetic easy axis.

In Fig. S5 we show the reversal process of the NFO//MGO (001) sample utilizing the LSSE measurements at selected angles of the external magnetic field  $\phi$  (see Fig. 1(b) and Fig. S2(b)). Similar to the NFO//CGO (011) sample presented in Fig. S4, the NFO//MGO (001) sample shows a dominant fourfold anisotropy with a magnetic easy axis along the  $\phi = 45^\circ$  direction relative to the magnetic harder directions along  $[100]$  and  $[010]$ . Again we see a switching of the magnetization along or close to the magnetic easy axis comparable to the switching process of NFO//CGO (011) which is expected due to the similar four-fold in-plane anisotropy. Here, the absence of the additional two-fold anisotropy has a minor impact on the reversal process given that a  $\sim 4\%$  reduction of the in-plane resonance field  $H_{\text{res}}$  on account of the additional weak uniaxial magnetic anisotropy of the NFO//CGO (011) sample is almost negligible compared to the NFO//MGO (001) sample shown here (cf. Fig. 3(b) of the Main Text and Fig. S6). The magnetization is in saturation at the beginning and end of the reversal process and in the same way switches when the magnetization has coherently rotated up to  $\sim 15^\circ$  relative to the magnetic easy axis.

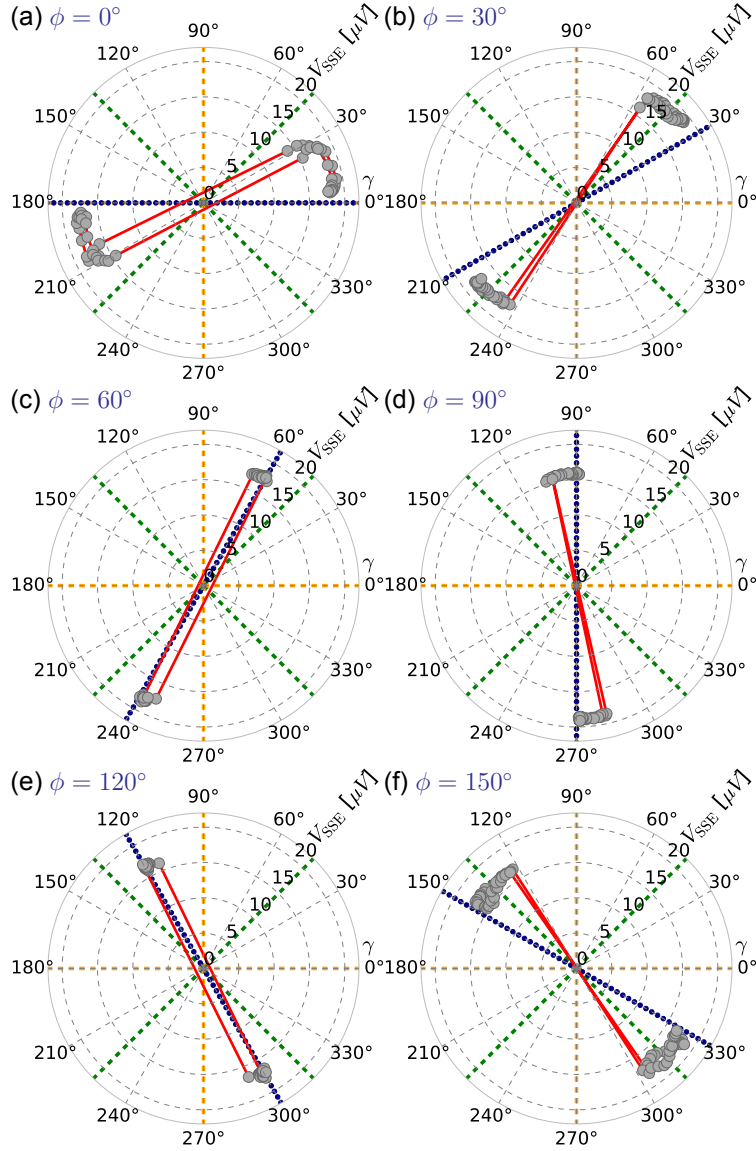

FIG. S4. (Color online) The NFO//CGO (011) reversal processes of the magnetization vector for angles of the external magnetic field (blue dotted line)  $\phi$  from  $0^\circ$  to  $150^\circ$  ((a) - (f)) relative to the [100] in-plane direction (see Main Text insert Fig. 2(a)). The magnitude of the magnetization vector given by  $|V|$  of the combined LSSE measurements in  $\mu\text{V}$  is plotted against the rotation angle  $\gamma$  of the magnetization vector. The magnetic easy (green) and magnetic hard axes (orange) are marked by dashed lines.

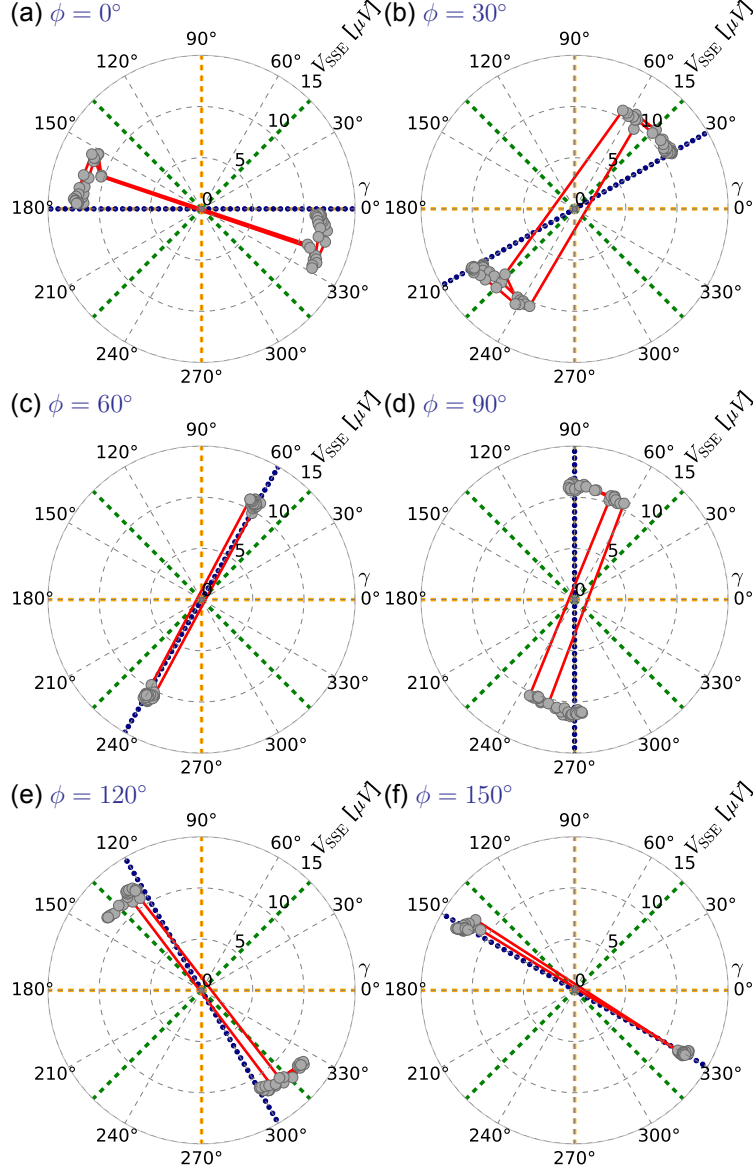

FIG. S5. (Color online) The NFO/MGO (001) reversal processes of the magnetization vector for angles of the external magnetic field (blue dotted line)  $\phi$  from  $0^\circ$  to  $150^\circ$  ((a) - (f)) relative to the [100] in-plane direction (see the inset Fig. S2(a)). The magnitude of the magnetization vector given by  $|V|$  of the combined LSSE measurements in  $\mu V$  is plotted against the rotation angle  $\gamma$  of the magnetization vector. The magnetic easy (green) and magnetic hard axes (orange) are marked by dashed lines.

## VI. FMR results for NFO//MGO (011), NFO//CGO (011) and NFO//MGO (001)

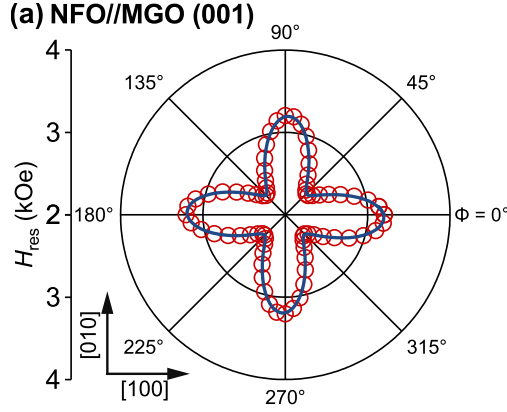

FIG. S6. (Color online) FMR measurements of the in-plane angular dependence of the resonance field,  $H_{\text{res}}$ , at 20 GHz for NFO//MGO (001) (see Main Text Fig. 3 for NFO//MGO (011) and NFO//CGO (011)).

Ferromagnetic resonance measurements were performed on 450 nm thick NFO films grown on (001)- and (011)-oriented MGO and CGO substrates with the external magnetic field applied in the plane of the sample.

The resonance field ( $H_{\text{res}}$ ) as a function of the in-plane rotation angle  $\phi$  shows four-fold symmetry for films grown on MGO (001) substrates having [100] and [010] as in-plane magnetic hard axes. Films grown on MGO (011) and CGO (011) substrates both show a four-fold magnetic anisotropy, in addition to a strong uniaxial magnetic anisotropy in NFO//MGO (011) and a weak uniaxial magnetic anisotropy in NFO//CGO (011) (Fig. S6 & S7 as well as Fig. 3 of the Main Text). The data was fit to the Smit-Beljers equation [1]

$$\left(\frac{\omega}{\gamma_g}\right)^2 = \frac{1}{M_s \sin^2 v} \left[ \frac{\partial^2 F}{\partial v^2} \frac{\partial^2 F}{\partial \gamma^2} - \left( \frac{\partial^2 F}{\partial v \partial \gamma} \right)^2 \right], \quad (\text{S2})$$

where  $\omega = 2\pi f$  is the angular frequency of the microwave field,  $M_s$  is the saturation magnetization,  $\gamma_g$  is the gyromagnetic ratio,  $v$  is the polar angle with respect to the normal of the film and  $\gamma$  is the azimuthal angle of the magnetization. Equation (S2) is evaluated at the equilibrium  $(v_0, \gamma_0)$  of the magnetization, which means

$$\left. \frac{\partial F}{\partial v} \right|_{v_0} = 0 \text{ and } \left. \frac{\partial F}{\partial \gamma} \right|_{\gamma_0} = 0. \quad (\text{S3})$$

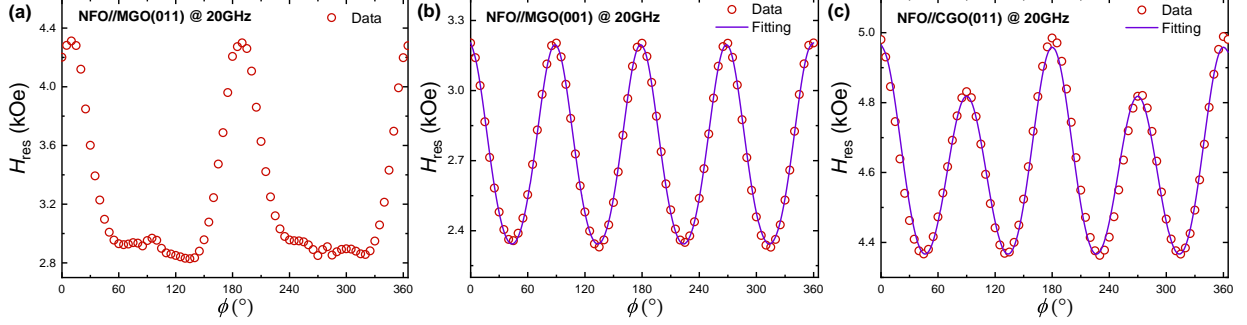

FIG. S7. (Color online) Full 360 degree in-plane rotation plots for (a) NFO/MGO (011), (b) NFO/MGO (001) and (c) NFO/CGO (011), respectively. The films grown on MGO (011) and CGO (011) substrate show a four-fold and a strong or weak two-fold magnetic anisotropy, while the film grown on MGO (001) substrate only shows a four-fold magnetic anisotropy. The purple lines are a fit to the data using the Smit-Beljers equation.

The total energy per unit volume is modeled as

$$F = -H_0 M_s [\sin v_M \sin v_H \cos(\gamma_H - \gamma_M) + \cos v_M \cos v_H] - \left(2\pi M_s^2 - K_U^\perp\right) \sin^2 v_M K_U^\parallel \cos^2 \gamma_M \sin^2 v_M - \frac{K_1}{8} [3 + \cos 4(\gamma_M - \gamma_U)], \quad (\text{S4})$$

where the terms in the equation above are Zeeman energy, uniaxial perpendicular magnetic anisotropy, in-plane uniaxial magnetic anisotropy and in-plane four-fold magnetic anisotropy energy, respectively. In our case  $v_M = v_H = 90^\circ$ .

The values of constants obtained by the fit is summarized in Table S1. Data for the film grown on MGO (011) substrate could not be fit due to scattered data around  $90^\circ$  and  $270^\circ$ .

The effective magnetization  $M_{\text{eff}}$  and gyromagnetic ratio  $\gamma_g' (= \frac{\gamma_g}{2\pi})$  in the equation below

$$f = \gamma_g' \sqrt{\left[H_{\text{res}} + H_U^\parallel \cos(2\gamma) + H_4 \cos(4\gamma)\right] \left[H_{\text{res}} + 4\pi M_{\text{eff}} + H_U^\parallel (\cos \gamma)^2 + \frac{H_4}{4} (3 + \cos(4\gamma))\right]} \quad (\text{S5})$$

are determined by broadband FMR measurement along in-plane magnetic easy axis and hard axis, and the data is simultaneously fitted using the Kittel equation [2] (Eq. (S4)), by fixing  $\gamma = 0^\circ$  for the magnetic hard axis and  $\gamma = 45^\circ$  for the magnetic easy axis.

For the film grown on CGO (011), the FMR measurement is done along in-plane [100] and [010] direction and the data is fit using the Kittel equation above (Eq. (S4)) by fixing  $\gamma = 0^\circ$  and  $\gamma = 90^\circ$ . Lastly, for the film grown on MGO (011), the FMR measurement is done in out-of-plane configuration. The parameters extracted from in-plane rotation measurement agree with the parameters obtained from broadband measurement and also the results from the VSM measurement.

TABLE S1. Details of the fitted data of the FMR measurements for all three samples NFO//MGO (011), NFO//CGO (011), and NFO//MGO (001).

|                | $H_s$<br>[kOe]    | $4\pi M_{\text{eff}}$<br>[kG] |                      | $4\pi M_s$<br>[kG] |       | $\gamma'$<br>[MHz/Oe] | $H_U^\perp$<br>[kOe] | $H_4$<br>[Oe] |                  | $H_U^\parallel$<br>[Oe] | $\alpha_{\text{eff}}$       |
|----------------|-------------------|-------------------------------|----------------------|--------------------|-------|-----------------------|----------------------|---------------|------------------|-------------------------|-----------------------------|
|                | VSM <sup>a)</sup> | ip-rot <sup>b)</sup>          | Kittel <sup>c)</sup> | ip-rot             | VSM   | Kittel                | ip-rot               | ip-rot        | Kittel           | ip-rot                  |                             |
| NFO//MGO (011) | 12.5              | -                             | 9.6<br>$\pm 0.03$    | -                  | 3.292 | 3.09<br>$\pm 0.02$    | -                    | -             | -                | -                       | 4.9E-3 <sup>d)</sup>        |
| NFO//CGO (011) | 5.25              | 4.632                         | 4.5<br>$\pm 0.3$     | 2.211              | 2.035 | 3.1<br>$\pm 0.01$     | 2.421                | -357          | -364<br>$\pm 64$ | 106<br>$\pm 8$          | 5.4E-4<br>$\pm 8\text{E-}5$ |
| NFO//MGO (001) | 15                | 12.929                        | 13.24<br>$\pm 0.05$  | 3.129              | 2.701 | 3.076<br>$\pm 0.004$  | 9.8                  | -482          | -474<br>$\pm 3$  |                         | 7.9E-4<br>$\pm 6\text{E-}5$ |

a): from VSM measurement.

b): from in-plane rotation measurement.

c): from Kittel plot.

d):  $\alpha_{\text{max}}$

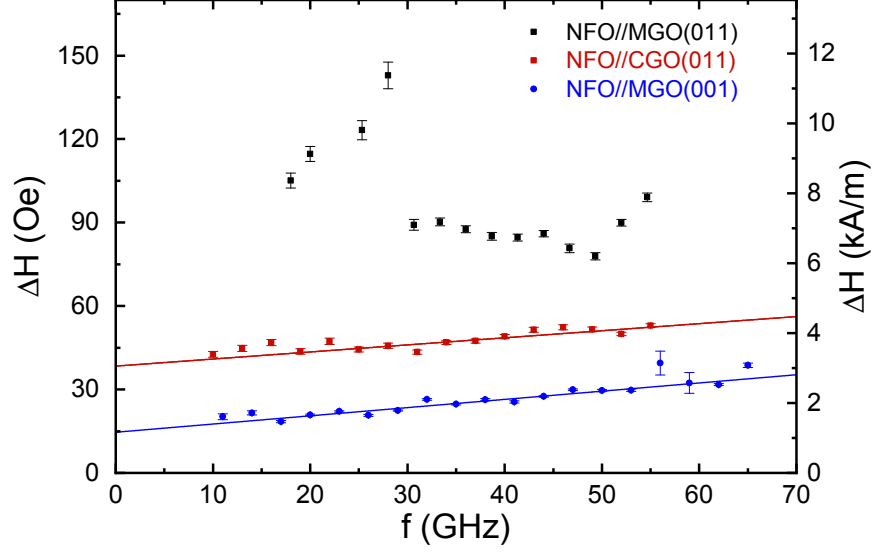

FIG. S8. (Color online) Linewidth vs frequency plot of all the films. The continuous line is a fit to the data using Eq. (S6). Data points for NFO//CGO (011) and NFO//MGO (001) at frequencies lower than 20 GHz were excluded from the fitting as the linewidth get broadened due to merging of multiple resonances with the main resonance.

As shown in Fig. S8, the linewidth of the NFO//MGO (011) film ( $\sim 99$  Oe at 55 GHz) is the highest among all the samples, and its linewidth vs frequency is also not linear, thus we get a maximum damping constant ( $\alpha_{\max} = 4.9 \times 10^{-3}$ ) for this sample. In contrast, the linewidths of the other two samples are much less ( $\sim 53$  Oe for NFO//CGO (011),  $\sim 40$  Oe for NFO//MGO (001) all at 55 GHz). Moreover, the damping constants  $\alpha_{\text{eff}}$  [3] of these samples, calculated from

$$\Delta H = \Delta H_0 + \frac{2}{\sqrt{3}} \times \alpha \times \frac{f}{\gamma_g'}, \quad (\text{S6})$$

are of the order of  $10^{-4}$ , mentioned in Table S1. It also shows that the minimum value ( $5.4 \times 10^{-4} (\pm 8 \times 10^{-5})$  for NFO//CGO (011) and  $7.9 \times 10^{-4} (\pm 6 \times 10^{-5})$  for NFO//MGO (001)).

## References

- [1] J. Smith and H.G. Beljers, Phillips Res. Rep 10 (2), 113 (1955).
- [2] C. Kittel, Physical Review 73 (2), 155 (1948).
- [3] C. Mewes and T. Mewes, in Handbook of Nanomagnetism (Pan Stanford, 2015), pp.71.
